# Supplementary material for: Discriminative models for robust image classification
Source: arXiv:1603.02736 source file (2016-03-08)
Supplement: Supplementary file 3 [file Dedication.tex]

% Place the dedication below.

To my parents, my grandparents, and all my teachers.
