# Supplementary material for: Discriminative models for robust image classification
Source: arXiv:1603.02736 source file (2016-03-08)
Supplement: Supplementary file 4 [file ListOfSymbols.tex]

% Place the list of symbols below.
\begin{eqlist}[\labelsep 1em]

\item[$\alpha$]
The first greek letter, p.~\pageref{}

\item[$\alpha$]
The first greek letter, p.~\pageref{}

\item[$\alpha$]
The first greek letter, but we should really add some more text, though we need it to go on two lines, p.~\pageref{}

\item[$\alpha$]
The first greek letter, p.~\pageref{}

\item[$\alpha$]
The first greek letter, p.~\pageref{}

\item[$\alpha$]
The first greek letter, p.~\pageref{}

\item[$\alpha$]
The first greek letter, p.~\pageref{}

\item[$\alpha$]
The first greek letter, p.~\pageref{}

\end{eqlist}
